# Supplementary material for: Equation of State and Progenitor Dependence of Stellar-Mass Black-Hole Formation
Source: arXiv:2001.10434 source file (2020-01-28)
Supplement: Supplementary file 1 [file appendix.tex]

\section{Effective Potentials}
\label{appendix}

\begin{figure*}[!htb]
\plotone{{figures/swh18_mass}.pdf}
\vspace{-0.25cm}
\caption{\label{fig:GR_GREP_mr} Comparison of PNS mass, PNS radius, and shock radius evolution for full GR simulations using \textsc{GR1D} (top plots) and the deviation of the different GREP approximations using \textsc{Flash} from the full GR run (bottom plots). 
We limit the plot to 4 models for clarity. 
Other models tested exhibit similar qualitative and quantitative behaviors. 
Deviations of observable $X$ computed using the GREP approximation with respect to the full GR approach are given by $\sigma_X=1-X^{GREP}/X^{\rm GR}$. 
Soon after bounce, $0.02\unit{s}\lesssim t-t_\rbounce \lesssim 0.2\unit{s}$, all GREP models overestimate PNS masses by 2 to 7\%. 
At later times, $t-t_\rbounce \gtrsim 0.2\unit{s}$, the GREP1 and GREP2 models predict PNS mass that agree with GR calculations, while GREP3 underrates the PNS mass. 
GREP1 and GREP2 approaches predict deviations that are limited to $\sim5\%$ from the GR calculations for the PNS and shock radii. 
Radii in the GREP3 approximation deviates further from the GR values.}
\end{figure*}

We expand further on the differences between the results of a full GR calculation using \textsc{GR1D} and those using effective potentials in \textsc{Flash}, see Section~\ref{ssec:GREP}. 
First, we compare predictions for the PNS gravitational mass, its radius as well as the shock radius, for some progenitor models, see Figure~\ref{fig:GR_GREP_mr}. 
We also plot deviations of the GREP runs with respect to the GR calculations. 
We limit the plot to four pre-SN progenitors for clarity and note that both qualitative and quantitative behavior are quite similar for all other progenitors. 
Soon after bounce, $0.02\unit{s}\lesssim t-t_\rbounce \lesssim 0.20\unit{s}$, a deviation of order a few percent is observed between simulations using GR and the ones using GREP is observed for the PNS mass. 
Afterwards, up to the point of BH formation, the deviation in predicted PNS mass between GR and GREP approaches reduces to $\lesssim2\%$. 
While using the GREP1 and GREP2 potentials slightly overestimates the PNS masses, $\lesssim1\%$ with less compact models agree better with GR simulations, while the GREP3 approach overrates the PNS mass by $\simeq2\%$ at the end of the run for all pre-SN progenitors. 
Meanwhile, both PNS and shock radii are overestimated by up to $\simeq8\%$ throughout the run for the GREP1 and GREP2 models, while GREP3 overrates radii by an even larger amount, up to $\simeq16\%$.
Exceptions to this behavior sometimes occur; usually very early after bounce, $t-t_\rbounce \lesssim 0.02\unit{s}$, whenever a composition shell crosses the shock radius, and very close to BH formation times.

\begin{figure*}[!htb]
\plotone{{figures/swh18_nu}.pdf}
\vspace{-0.5cm}
\caption{\label{fig:GR_GREP_nu} Comparison of neutrino luminosities (first row) and RMS energy (third row) for electron neutrinos (left column), electron antineutrinos (center column), and heavy neutrinos (right column) for GR simulations using \textsc{GR1D}. 
Deviation of the different GREP approximations using \textsc{Flash} with respect to \textsc{GR1D} results for luminosity (second row) and RMS energy (fourth row) are also shown. 
We limit the plot to 4 different progenitor models for clarity. 
Other models tested exhibit similar qualitative and quantitative behaviors. 
Deviations of observable $X$ computed using the GREP approximation with respect to the full GR approach are given by $\sigma_X=1-X^{GREP}/X^{\rm GR}$. 
Deviations between GR and GREP approaches can be large soon after bounce, but reduce to the 5-10\% level throughout most of the run for electron neutrinos and anti-neutrinos. 
We note that deviations are usually larger for the GREP3 approach. 
Finally, deviations in luminosity for the heavy neutrinos become quite large at late times, being off up to a factor of 2 for the $18\,M_\odot$ progenitor model by BH formation time.}
\end{figure*}

In Figure~\ref{fig:GR_GREP_nu} we compare the neutrino luminosities and average root-mean-square (RMS) energies for electron neutrinos, electron antineutrinos, and heavy neutrinos in the GREP approximations with the results from GR simulations. 
We note that electron neutrino and antineutrino luminosities (RMS energies) are reproduced in the GREP within 5 to 10\% (2 to 4\%) of the GR computed values. 
Again, as in the shock radius the differences that arise between GR and GREP calculations are more extreme soon after core bounce, when a composition shell crosses the shock radius, and very close to BH formation times. 
While heavy neutrino RMS energies deviations between GR calculations and GREP approximation are often of similar magnitude to those of the electron-type neutrinos, except at the very end of each run, their luminosity can be quite different, with differences being as large as 50\% or more at the end of some runs. 
This is also observed by \citet{oconnor:18a} when comparing relativistic and non-relativistic simulation codes for the core collapse of a $20\,M_\odot$ star.
